# Supplementary material for: Self-assembly of 2D membranes from mixtures of hard rods and depleting polymers
Source: arXiv:1103.2760 ancillary file (2011-03-14)
Supplement: Supplementary file 1 [file paperSimulation.si.pdf]

# Supporting Information for: Self-assembly of 2D membranes from mixtures of hard rods and depleting polymers

## I. THE ORIGINS OF MEMBRANE-MEMBRANE REPULSIVE INTERACTIONS.

In this section we analyze in more detail the origin of the interactions that stabilize membranes against stacking, and we provide additional justification for the simplification of parallel rods in the simulation.

### A. The bending modulus is large

Fig. 1 compares the membrane height-height correlation functions for membranes composed of parallel rods and rods with orientational fluctuations. The calculation details are outlined in section II below. We observe that, for all the wavelengths allowed the fluctuation spectrum scales with wave number $1/q^2$ in both cases. For parallel rod membranes this scaling is forced by construction [1]. In contrast for membranes with orientation degrees of freedom rods, $1/q^2$ scaling arises because the large rod aspect ratio of constituent rods leads to a high bending modulus. The $q$-dependence of the fluctuation spectrum reflects a superposition of bending and protrusion modes, according to $S \sim \frac{k_\mathrm{B}T}{\gamma q^2} + \frac{k_\mathrm{B}T}{\kappa_\mathrm{c} q^4}$ [2], with $\gamma$ the surface tension and $\kappa_\mathrm{c}$ the bending modulus. The $q^4$ dependence should dominate for wave numbers smaller than $q_\mathrm{c} \cong (\gamma/\kappa_\mathrm{c})^{1/2}$ [2]. The large magnitude of the bending modulus can be understood to arise from the large aspect ratio of our rods based on the scaling arguments in Ref. [2]. There it is shown that the bending modulus scales quadratically with membrane thickness; i.e., $\kappa_\mathrm{c} \sim L^2$.

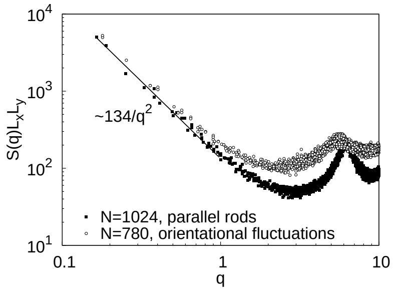


FIG. 1. Symbols: Height-height correlation spectrum for simulations with a single membrane of $N = 1024$ parallel rods, and a single membrane of $N = 780$ rods with orientational fluctuations. The parameters used are $\delta = 1.5$, $L = 100$ and $p_\mathrm{s} = 0.06$.

### B. Membrane-membrane interactions

For two flat plates, the depletion interaction is linear for small separations $d \leq \delta$, and negligible for $d > \delta$ [3]. However, the equivalent interaction occurs over a significantly longer range for membranes, due to fluctuations of constituent rods. These fluctuations have two effects on membrane-membrane interactions, which can be disentangled by separating the free energy into a depletion term and a term arising from rod protrusions, $f(d) = f_\mathrm{ex} + f_\mathrm{pr}$. The depletion term is given by $f_\mathrm{ex}(d) = p_\mathrm{s}\langle v_\mathrm{ex}(d)\rangle$, where $v_\mathrm{ex}$ is the volume excluded to spheres by rods, and $\langle\cdot\rangle$ indicates an ensemble average over configurations at a particular separation $d$. The excluded volume (per rod) is calculated for each particular system configuration as $v_\mathrm{ex} \approx (L_x L_y L_z - N_\mathrm{s}/\rho_\mathrm{s})/N$, with $N_\mathrm{s}$ the number of polymer spheres for that configuration. The protrusion term can then be calculated as $f_\mathrm{pr}(d) = f(d) - f_\mathrm{ex}(d)$. As shown in Fig. 2, the ranges of the depletion and protrusion interactions are comparable, and much larger than the sphere diameter. The enhanced interaction range occurs because membrane undulations bring rods in neighboring membranes within the bare depletion interaction range for large mean membrane separations.

The interaction between two membranes in which bending modes dominate over protrusions was derived by Helfrich [4–6]. The suppression of progressively smaller wavelength modes as membranes approach gives rise to a free energy per area

$$g_\mathrm{bend}(d) = \frac{3(k_\mathrm{B}T)^2}{2\pi^2\kappa_\mathrm{c}(d-L)^2}, \tag{1}$$

where $d - L$ is the mean separation between the surfaces of the two membranes.

We adapt the arguments of Helfrich and Servuss [5] to derive an analogous expression for the case in which protrusion modes dominate over bending modes as follows. We decompose the undulations $u(\mathbf{r})$ of an isolated membrane into modes, with the amplitude $u_q$ of a mode with wavelength $q$ given by the equipartition theorem

$$\langle |u_q|^2\rangle = \frac{k_\mathrm{B}T}{A\gamma q^2} \tag{2}$$

with $\gamma$ the surface tension and $A$ the membrane area. The mean squared amplitude of undulations is then given by a sum over modes, which we approximate with the integral

$$\langle u^2\rangle = \frac{k_\mathrm{B}T}{2\pi\gamma}\int_{q_\mathrm{min}}^{q_\mathrm{max}} \frac{dq}{q} \tag{3}$$

with the cutoff wave vectors $q_\mathrm{min} = \pi A^{-1/2}$ and $q_\mathrm{max} =$

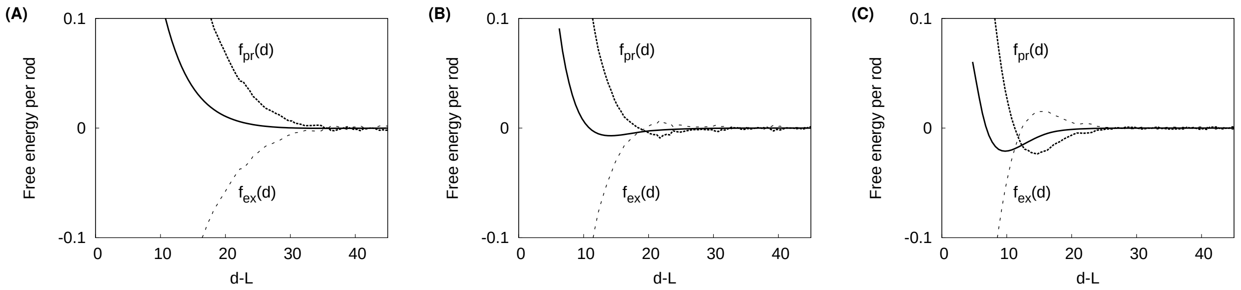


FIG. 2. The total free energy can be split into a depletion term and a term arising from rod protrusions,$f(d) = f_{\mathrm{ex}} + f_{\mathrm{pr}}$. The solid lines are $f(d)$, the dotted lines correspond to the protrusion interaction $f_{\mathrm{pr}}$, and the dashed lines correspond to the depletion interaction $f_{\mathrm{ex}}$. The rod length is $L = 100$, the sphere diameter is $\delta = 1.5$, and osmotic pressures are $p_{\mathrm{s}} = 0.06$, 0.09 and 0.12, from (A) to (C), respectively.

$\pi/\sigma$ with $\sigma$ the particle diameter. The integral gives

$$\langle u^2 \rangle = \frac{k_{\mathrm{B}}T}{2\pi}\gamma \ln\left(\frac{A^{1/2}}{\sigma}\right). \tag{4}$$

The repulsive interaction between two membranes results because progressively more modes are suppressed as the membranes approach. Following Helfrich [5] we first consider a single membrane between two parallel rigid plates, which are respectively separated by $+d_{\mathrm{s}}$ and $-d_{\mathrm{s}}$ from the mean plane of the membrane. The plates provide a hard wall interaction that restricts undulations to

$$-d_{\mathrm{s}} < u(\mathbf{r}) < d_{\mathrm{s}}. \tag{5}$$

While the complete effect of this confinement on the mode structure is complicated, restricting $-d_{\mathrm{s}} < u(\mathbf{r}_0) < d_{\mathrm{s}}$ at one point $\mathbf{r}_0$ results in

$$\langle u^2(\mathbf{r}_0)\rangle = d_{\mathrm{s}}^2/3 \tag{6}$$

while exciting a single mode with wavelength $q$ and then restricting $-d_{\mathrm{s}} < u(\mathbf{r}) < d_{\mathrm{s}}$ for all $\mathbf{r}$ results in

$$\langle u_q^2(\mathbf{r})\rangle = d_{\mathrm{s}}^2/12. \tag{7}$$

The mean squared displacement of a membrane for which all modes can be excited, but is confined to the interval Eq. 5 for all $\mathbf{r}$ is then approximated by the geometric mean [5]

$$\langle u_q^2(\mathbf{r})\rangle = d_{\mathrm{s}}^2/6. \tag{8}$$

We then insert Eq. 8 into Eq. 4 and solve for $A$. The system of one membrane between two rigid plates separated by distance $2d_{\mathrm{s}}$ is equivalent to two membranes with mean separation between their surfaces $d_{\mathrm{s}}$ and each with surface tension $\gamma/2$ [4]. We thus obtain

$$A_{\mathrm{coll}} = \sigma^2 \exp\left(\frac{\pi}{3}\frac{\gamma d_{\mathrm{s}}^2}{k_{\mathrm{B}}T}\right), \tag{9}$$

where $A_{\mathrm{coll}}$ gives the average area per membrane-membrane collision. Assuming as usual that each collision results in a free energy of $k_{\mathrm{B}}T$, the total interaction free energy is given by the number of collisions:

$$g_{\mathrm{pr}}(d) = B \exp\left[-\frac{\pi}{3}\frac{\gamma(d-L)^2}{k_{\mathrm{B}}T}\right], \tag{10}$$

with $B$ a pre-factor of order (1), and $g_{\mathrm{pr}}$ is defined as the free energy per unit area, and we used $d_{\mathrm{s}} = d - L$. The free energy per rod is then $f_{\mathrm{pr,theory}} = (2\rho_{\mathrm{2d}})^{-1} g_{\mathrm{pr}}$, with $\rho_{\mathrm{2d}}$ the areal density of rods in the membrane. An expression with a similar functional form is derived in Lipowsky and Fischer [7].

As shown in Fig. 3, the measured membrane-membrane interaction potential is well fit by the functional form of Eq. 10 for a range of parameter values. We note however that the fits require an effective value of the surface tension that is close to, but consistently smaller than, the actual value extracted from fluctuation correlation spectra. For example, with $p_{\mathrm{s}} = 0.06$ the measured value of surface tension is $\gamma\sigma^2 \approx 1/134$ (Fig. 1) while the best fit value in Fig. 3 is $\gamma\sigma^2 = 1/213$. The small discrepancies could arise from the crudity of the arguments leading to Eq. 8. Thus, we also adapted a different calculation for the interactions due to bending modes, described in Ref. [4] and Chapter 6.6 of Ref. [6], to the case in which protrusions dominate. This calculation, which starts with the energy for a system of membranes with smectic order, resulted in an expression (valid for large $d - L$)

$$\hat{g}_{\mathrm{pr}}(d) = \left(\frac{1}{6}\frac{\gamma d^2}{\sigma^2} + \frac{7\pi}{144}\frac{k_{\mathrm{B}}T}{\sigma^2}\right) e^{-1/2} \exp\left[-\frac{4}{\pi}\frac{\gamma(d-L)^2}{k_{\mathrm{B}}T}\right]. \tag{11}$$

This expression has a decay length which is almost identical to that of Eq. 10, and fitting to the data yields similar estimates for the surface tension, which supports the crude arguments given above.

We thus consider two likely origins of the discrepancies between apparent and measured surface tensions. First, membrane undulations are a superposition of collective protrusion modes and smaller scale individual rod protrusions. In particular the distribution of protrusions (Fig. 4) is Gaussian at small distances from the membrane surface, consistent with the continuum model, but

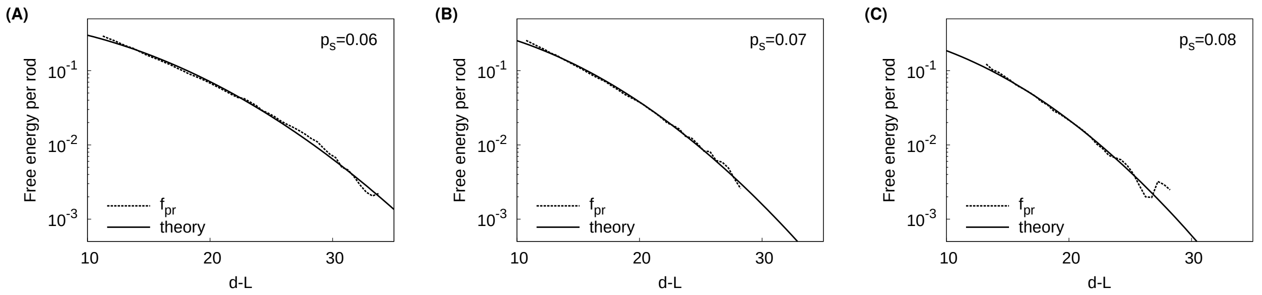


FIG. 3. The protrusion interaction potential is well-fit by the theory in some parameter ranges. The dotted lines show the repulsive interaction potential $f_{\rm pr}$ measured from simulations (Fig. 2), and the solid lines correspond to the best fit to $f_{\rm pr,theory}$ with $B$ and $\gamma$ as fit parameters. Parameters are $L = 100$, $\delta = 1.5$ and (A) $p_{\rm s} = 0.06$, (B) $p_{\rm s} = 0.07$, (C) $p_{\rm s} = 0.08$. The best fit parameters are (A) $B = 0.8$, $\gamma = 1/213$, (B) $B = 0.9$, $\gamma = 1/156$, and (C) $B = 0.7$, $\gamma = 1/146$.

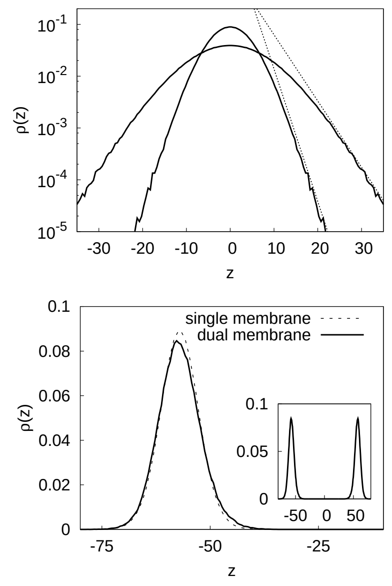


FIG. 4. (Top) Rod center distribution (protrusion distribution) in single membranes at osmotic pressures $p_{\rm s} = 0.06$(inner) and $p_{\rm s} = 0.12$(outer). The dashed lines indicate that the distributions approach $\sim \exp(\frac{1}{4}\pi(\delta+\sigma)^2 p_{\rm s}|z|)$ at large $|z|$. (Bottom) Rod center distribution of dual membranes at separation $d - L \approx 14$ and osmotic pressure $p_{\rm s} = 0.12$. The dashed line is the rod center distribution of a single membrane. The insertion shows the whole distribution. For both plots, parameters are $L = 100$, $\delta = 1.5$.

has an exponential tail consistent with individual protrusions [8]. It is possible that individual protrusions enhance the range of the interaction and thus reduce the best fit value of the surface tension.

Second, the attractive depletion interactions can expand the range of protrusions as membranes approach, resulting in a lower apparent surface tension. For example, for $p_{\rm s} = 0.12$ in Fig. 2, there is a intermediate distance range $d - L \in [13, 20]$, where $f_{\rm ex}(d)$ becomes positive; i.e., the excluded volume is larger then the value for membranes with infinite separation, while at the same time the total free energy is lower. At this intermediate distance range, the protrusion susceptibility is increased because the favorable entropy of protrusions is partially offset by partial overlap of excluded volume regions with rods from the opposing membrane. This result emphasizes that the depletion and protrusion forces are intimately coupled in the membrane interaction potential.

### C. Bending modes vs. protrusion modes

Comparison between Eq. 1 and the simulated membrane-membrane interactions further justifies the simplification of parallel rods in our simulations. As shown in Fig. 5, the predicted contribution of bending modes to the membrane-membrane interaction is several orders of magnitude smaller than the measured value due to protrusions. Note that the simulation free energy per rod $f_{\rm pr}$ is multiplied by $2\rho_{\rm 2d}$ to obtain a free energy per area. For this estimate, we used the experimentally measured value $\kappa_{\rm c} = 150 k_{\rm B}T$. While the actual bending modulus in simulations with orientational fluctuations is likely different, it is clear that protrusion modes will dominate regardless of the exact bending modulus.

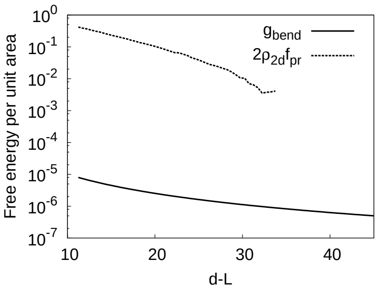


FIG. 5. The contribution to membrane-membrane interaction free energies due to bending modes predicted by Eq. 1 (solid line) is compared to the protrusion interaction free energy measured for membranes with parallel rods (dotted line). Parameters are $L = 100$, $\delta = 1.5$, and $p_{\rm s} = 0.06$.

## II. MEASUREMENT OF THE HEIGHT-HEIGHT CORRELATION SPECTRUM

We calculate the membrane height-height correlation function (flicker spectrum) of membranes using[9, 10]

$$S(\mathbf{q}) = \langle c_{\mathbf{n}} c_{\mathbf{n}}^* \rangle \tag{12}$$

where $\mathbf{q}$ is the wavevector,

$$\mathbf{q} = 2\pi \left( \frac{n_x}{L_x}, \frac{n_y}{L_y} \right) \tag{13}$$

and the amplitude $c_{\mathbf{n}}$ is given by

$$c_{\mathbf{n}} = \frac{1}{N} \sum_{i=1}^{N} (z_i - \bar{z}) \exp(-2\pi \mathrm{i}(q_x x_i + q_y y_i)) \tag{14}$$

with $\bar{z} \equiv N^{-1} \sum_i z_i$. As shown in Fig. 1, the spectrum is proportional to $1/q^2$ at long wavelengths. The effective surface tension $\sigma_{\mathrm{pr}}$ can be extracted from the relation

$$S(\mathbf{q}) = \frac{k_{\mathrm{B}}T}{\sigma_{\mathrm{pr}} L_x L_y q^2} \tag{15}$$

which gives $\sigma_{\mathrm{pr}} \approx 134 k_{\mathrm{B}}T/\sigma^2$ for $\delta = 1.5$, $L = 100$ and $p_{\mathrm{s}} = 0.06$, the case shown in Fig. 1. The peak at large $q$ arises from the first peak of radial distribution function shown in Fig. 6.

## III. MEMBRANE CRYSTALLIZATION

As noted in the main text, the simulated membranes crystallize for large osmotic pressures and aspect ratios. Crystallized membranes associate at lower osmotic pressures because they experience lower protrusion free energies $f_{\mathrm{p}}$. Due to the translational order of rods, two crystallized membranes can approach in such a way that each rod interacts with only one rod in the neighboring membrane. In contrast, when two liquid membranes approach each protruding rod in general interacts with several rods of the neighboring membrane. Consequently, there is a kink in the free energy as a function of osmotic pressure at the point of crystallization, above which the free energy decreases rapidly. We note that our simulations overestimate this effect because crystallized membranes are always aligned with the box directions due to the periodic boundary conditions, which eliminates one rotation required to achieve alignment. Furthermore, we find that larger aspect ratios and/or osmotic pressures are required for membranes to crystallize with orientational fluctuations enabled. Finally, the effect of crystallization on membrane-membrane interaction free energies would be unlikely to be seen experimentally due to kinetic considerations, since large membranes rotate slowly.

The boundary between liquid and crystallized membranes, which is indicated by the dashed line in Fig. 3A of the main text, was determined from radial distribution functions $g(r)$ measured within the plane of membranes at each parameter set; crystallized membranes have a double-peak in the radial distribution function at $r \approx 2$ [11]. Typical examples of $g(r)$ for liquid and crystallized membranes are shown in Fig. 6. The location of the solid-liquid coexistence line can be understood from two-dimensional hard disk systems, which computational studies [12, 13] showed freeze at a areal density $\rho_{2\mathrm{d}} \approx 0.88$. The transition in our simulations occurs at an areal rod density of 0.88; the relationship between osmotic pressure and areal rod density is theoretically calculated in Ref. [14].

There has been much discussion in the literature concerning the possibility that a hexatic phase precedes crystallinity in hard disk systems [15]. The number of rods in our membranes is far too small to investigate this possibility here, so we merely note that we see a direct transition from liquid to crystalline, which is consistent with large simulations of hard disks [11, 16, 17].

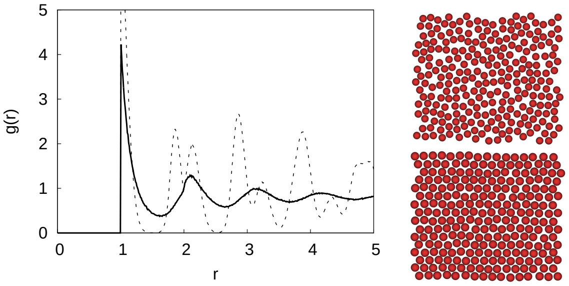


FIG. 6. (Left) Radial distribution functions of rods in the plane of membrane. The membrane is liquid at low surface density (Solid line, $\rho_{2\mathrm{d}} = 0.81$ at $p_{\mathrm{s}} = 0.06$), while at high surface density (Dashed line, $\rho_{2\mathrm{d}} = 0.98$ at $p_{\mathrm{s}} = 0.12$), a split double peak of $g(r)$ appears at $r \approx 2$ indicating the freezing of the membrane. (Right top) Cross section of a membrane at $p_{\mathrm{s}} = 0.06$. The membrane is a liquid. (Right bottom) Cross section of a membrane at $p_{\mathrm{s}} = 0.12$. The membrane is a solid. Rod length is $L = 100$.

## IV. FINITE SIZE EFFECTS

Since the phase diagrams are determined from simulations with $N = 256$ rods per membrane, it is important to verify that the phase boundaries are insensitive to $N$. To this end, we calculated membrane-membrane interaction free energies $f(d)$ as described above at a variety of osmotic pressures and rod lengths for membranes with $N$ = 64, 144, 256, 400 and 576. As shown in Fig. 7 A, for repulsive membranes, the free energy stays repulsive irrespective of membrane sizes, despite stronger repulsion for larger membrane sizes. For attractive liquid membranes, $F$ increases (i.e. the attractive basin gets shallower) with increasing $N$. For attractive crystallized membranes, $F$ decreases (i.e. the attractive basin gets deeper) with increasing $N$. However, the calculated

isolated-smectic and liquid-solid boundaries are insensitive to system size for $N \geq 144$, justifying our choice of 256 rods per membrane.

The finite size dependence of the interaction free energy of crystallized membranes can be understood as follows. Two crystallized membranes can decrease their protrusion free energy by aligning their hexagonal lattices as described above. This alignment is unfavorable entropically since it restricts one the global translational degree of freedom. This alignment restricts one translational degree of freedom, and thus increases the free energy per rod by a factor $\sim k_{\mathrm{B}}T/2N$. Indeed, the basin depth for $L = 100$ and $p_{\mathrm{s}} = 0.12$, can be fit against

$$\min(f_N) = f_0 + k k_{\mathrm{B}} T/2N \tag{16}$$

with factor $k \approx 1.7$, as shown in Fig. 7.

*Estimation of the finite size effect.* An upper bound for the pre-factor $k$ in Eq. 16 can be estimated from the precision with which rods are forced to align as: $k_{\mathrm{bound}} = \ln(A_0/A_1)$, with $A_0 = 1/\rho_{\mathrm{2d}}$ the area of unit cell of the lattice, and $A_1$ is the free area for one rod when its neighbors are fixed at their lattice sites. We calculate $A_1 = 12(\frac{1}{4}dc - \frac{1}{2}\arcsin\frac{c}{2})$, with $d = \sqrt{2/\sqrt{3}\rho_{\mathrm{2d}}}$ and $c = \frac{1}{2}(\sqrt{3}b - \sqrt{4-b^2})$. From simulations with parameters $L = 100$ and $p_{\mathrm{s}} = 0.12$ we measure $\rho_{\mathrm{2d}} \approx 0.98$, which gives $k_{\mathrm{bound}} \approx 3.6$. The actual value $k < k_{\mathrm{bound}}$ because rods are not perfectly aligned in optimal membrane configurations and there are regions where rods overlap with multiple partners in the opposing membrane.


[1] R. Lipowsky and S. Grotehans, Europhys. Lett. **23**, 599 (1993).
[2] R. Goetz, G. Gompper, and R. Lipowsky, Phys. Rev. Lett. **82**, 221 (1999).
[3] S. Asakura and F. Oosawa, J. Chem. Phys. **22**, 1255 (1954).
[4] W. Helfrich, Z. Naturforsch **33a**, 305 (1978).
[5] W. Helfrich and R. M. Servuss, Nuovo Cimento D **3**, 137 (1984).
[6] S. Safran, *Statistical Thermodynamics of Surfaces, Interfaces, and Membranes* (Addison-Wesley Pub., 1994).
[7] R. Lipowsky and M. E. Fisher, Phys. Rev. B **36**, 2126 (1987).
[8] J. N. Israelachvili and H. Wennerstrom, J. Phys. Chem. **96**, 520 (1992).
[9] W. K. den Otter and W. J. Briels, J. Chem. Phys. **118**, 4712 (2003).
[10] E. S. Boek, W. K. Den Otter, W. J. Briels, and D. Iakovlev, Phil. Trans. R. Soc. Lond. A **362**, 1625 (2004).
[11] T. M. Truskett, S. Torquato, S. Sastry, P. G. Debenedetti, and F. H. Stillinger, Phys. Rev. E **58**, 3083 (1998).
[12] H. Lowen, T. Palberg, and R. Simon, Phys. Rev. Lett. **70**, 1557 (1993).
[13] H. Weber, D. Marx, and K. Binder, Phys. Rev. B **51**, 14636 (1995).
[14] Y. Yang and M. F. Hagan, in preparation(2011).
[15] K. J. Strandburg, Rev. Mod. Phys. **60**, 161 (1988).
[16] E. Velasco and L. Mederos, Phys. Rev. B **56**, 2432 (1997).
[17] S. Luding, Phys. Rev. E **63**, 042201 (2001).

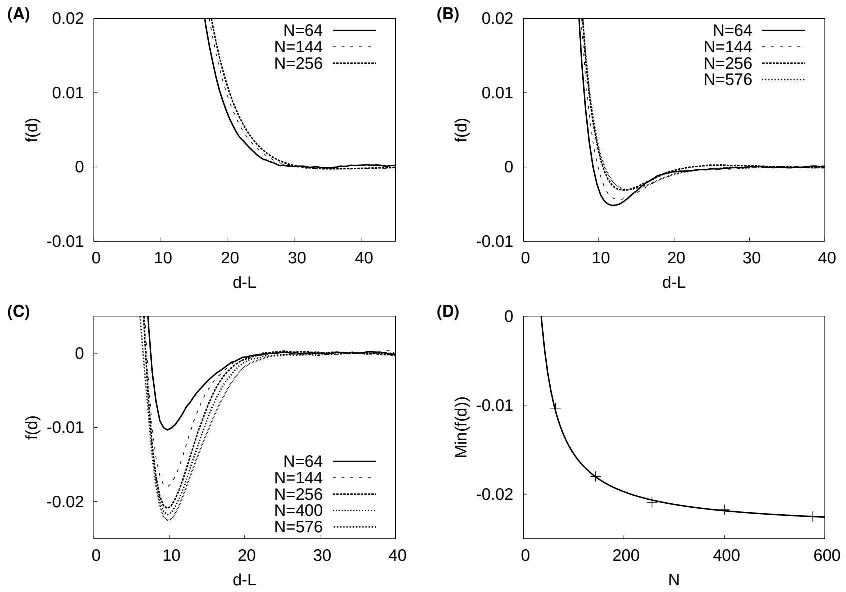


FIG. 7. Evaluation of finite size effects. (A)-(C) The free energy per rod $f(d)$ measured at membrane sizes $N = 64$, 144, 256, 400 and 576. Parameters are: (A) $L = 100$ and $p_{\rm s} = 0.06$, for which membranes are repulsive; (B) $L = 50$ and $p_{\rm s} = 0.12$, for which membranes are attractive but in the liquid phase; (C) $L = 100$ and $p_{\rm s} = 0.12$, for which membranes are attractive and crystallized. (D) The minima of $f(d)$ plotted in (C) v.s. membrane size $N$. Symbols are the simulation results. The line is the fit against $\min(f_N - f_\infty) = f_0 + k k_{\rm B} T/2N$, with fitting parameters $f_0 = -0.023$ and $k \approx 1.7$.
